# Supplementary material for: Team of One: Cracking Complex Video QA with Model Synergy
Source: arXiv:2507.13820 source file (2025-07-18)
Supplement: Supplementary file 1 [file X_suppl.tex]

\clearpage
\setcounter{page}{1}
\maketitlesupplementary

\section{Prompt Word}
\label{sup_sec:prompt}
The example of prompt words in three style (introduced in section \ref{subsec:prompt}) are show in Figure \ref{fig:prompt1}, \ref{fig:prompt2} and \ref{fig:prompt3}.
Among them, the underline indicates the content that needs to be filled based on the sample.
The italics indicate the corresponding guiding content, which can promote the large model to pay attention to some task related information that may have gains.
Symbol (...) indicates that some redundant text is omitted at this location.

It should be noted that in this work, we require VLM to output JSON format for easy access to the corresponding output section.
In order to constrain the standardization of the format, the prompt explicitly provides the required output format.
Additionally, the provided example also have a positive impact on formatting to some extent.

\begin{figure*}[b]
	\centering
	\includegraphics[width=.98\linewidth]{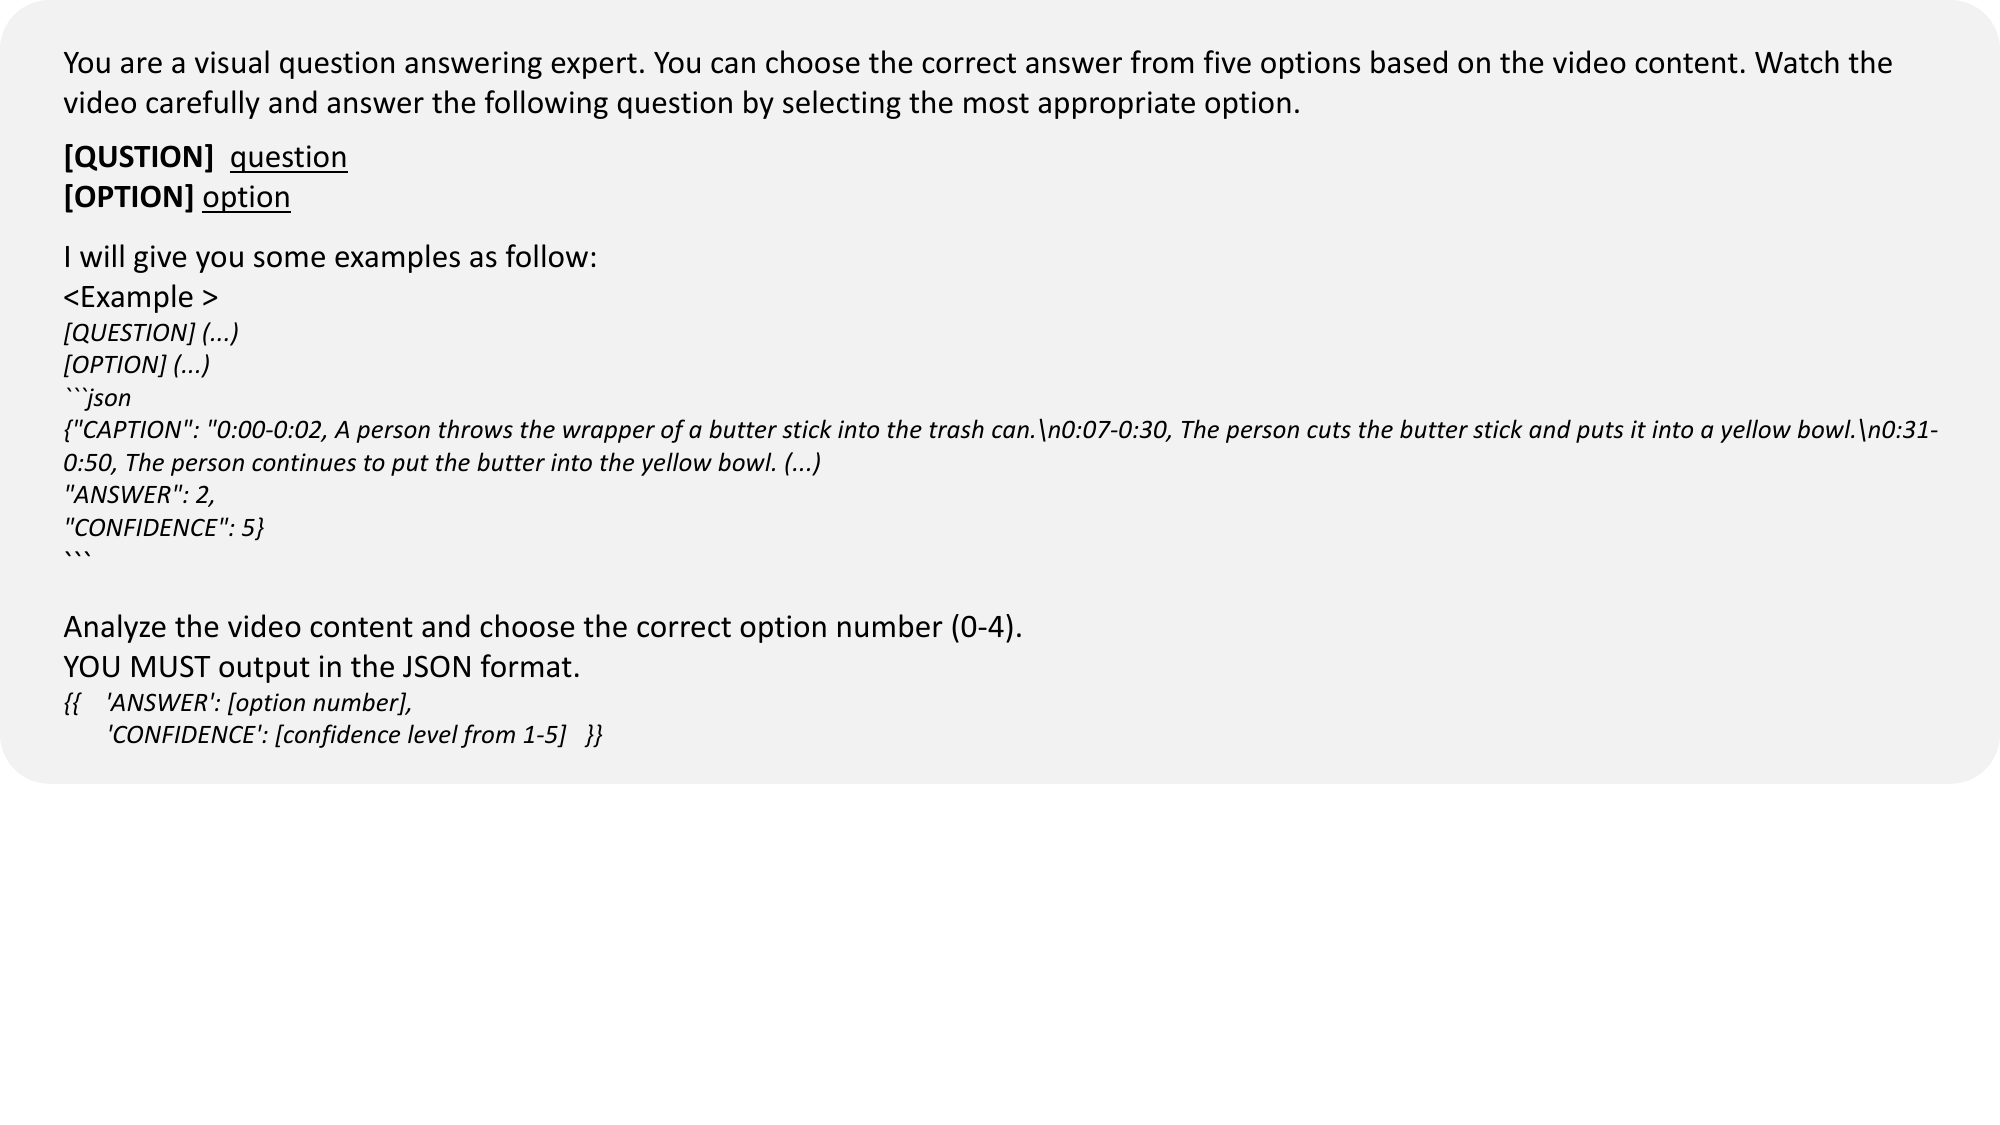}
	\caption{Example of prompt words in Style \textbf{P1}.}
	\label{fig:prompt1}
\end{figure*}

\begin{figure*}[ht]
	\centering
	\includegraphics[width=.98\linewidth]{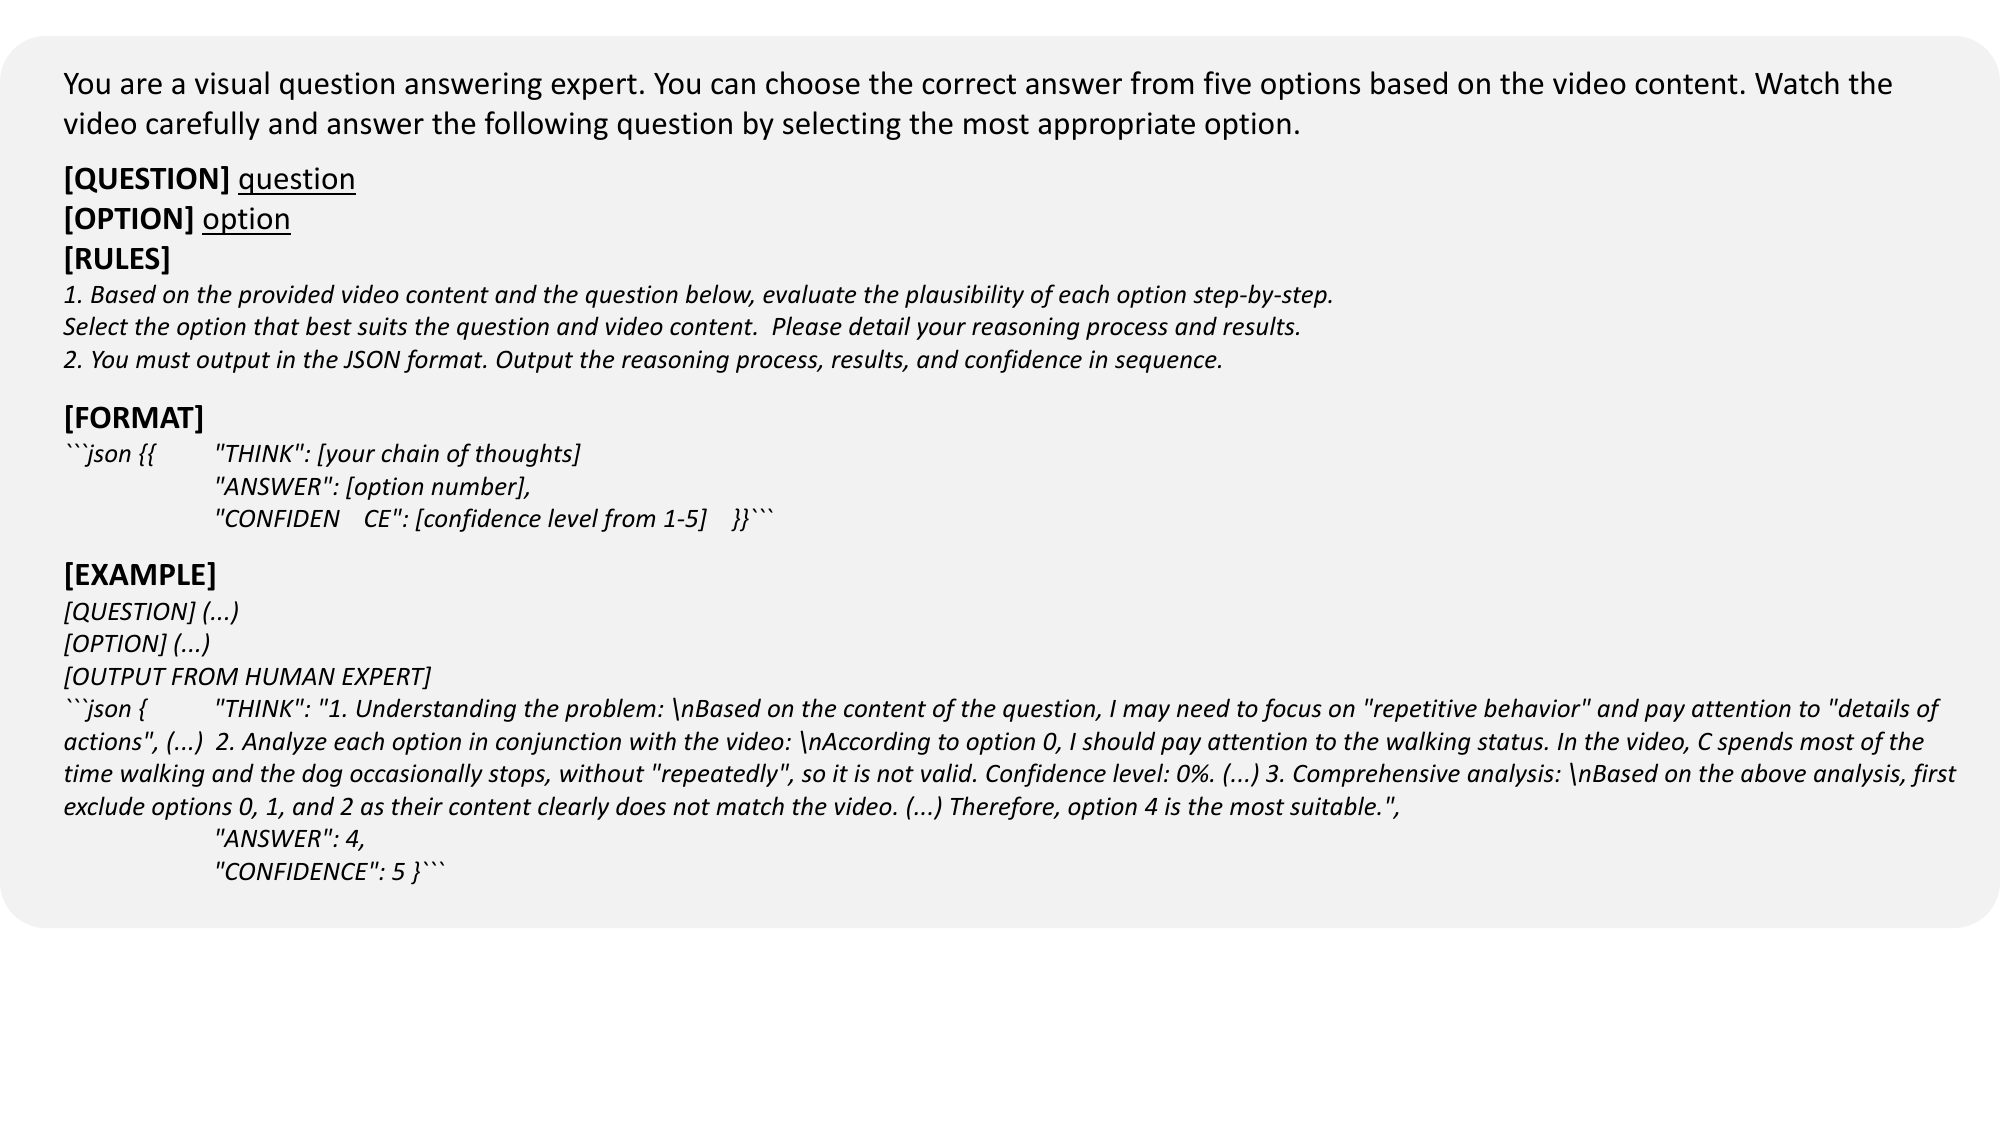}
	\caption{Example of prompt words in Style \textbf{P2}.}
	\label{fig:prompt2}
\end{figure*}

\begin{figure*}[ht]
	\centering
	\includegraphics[width=.98\linewidth]{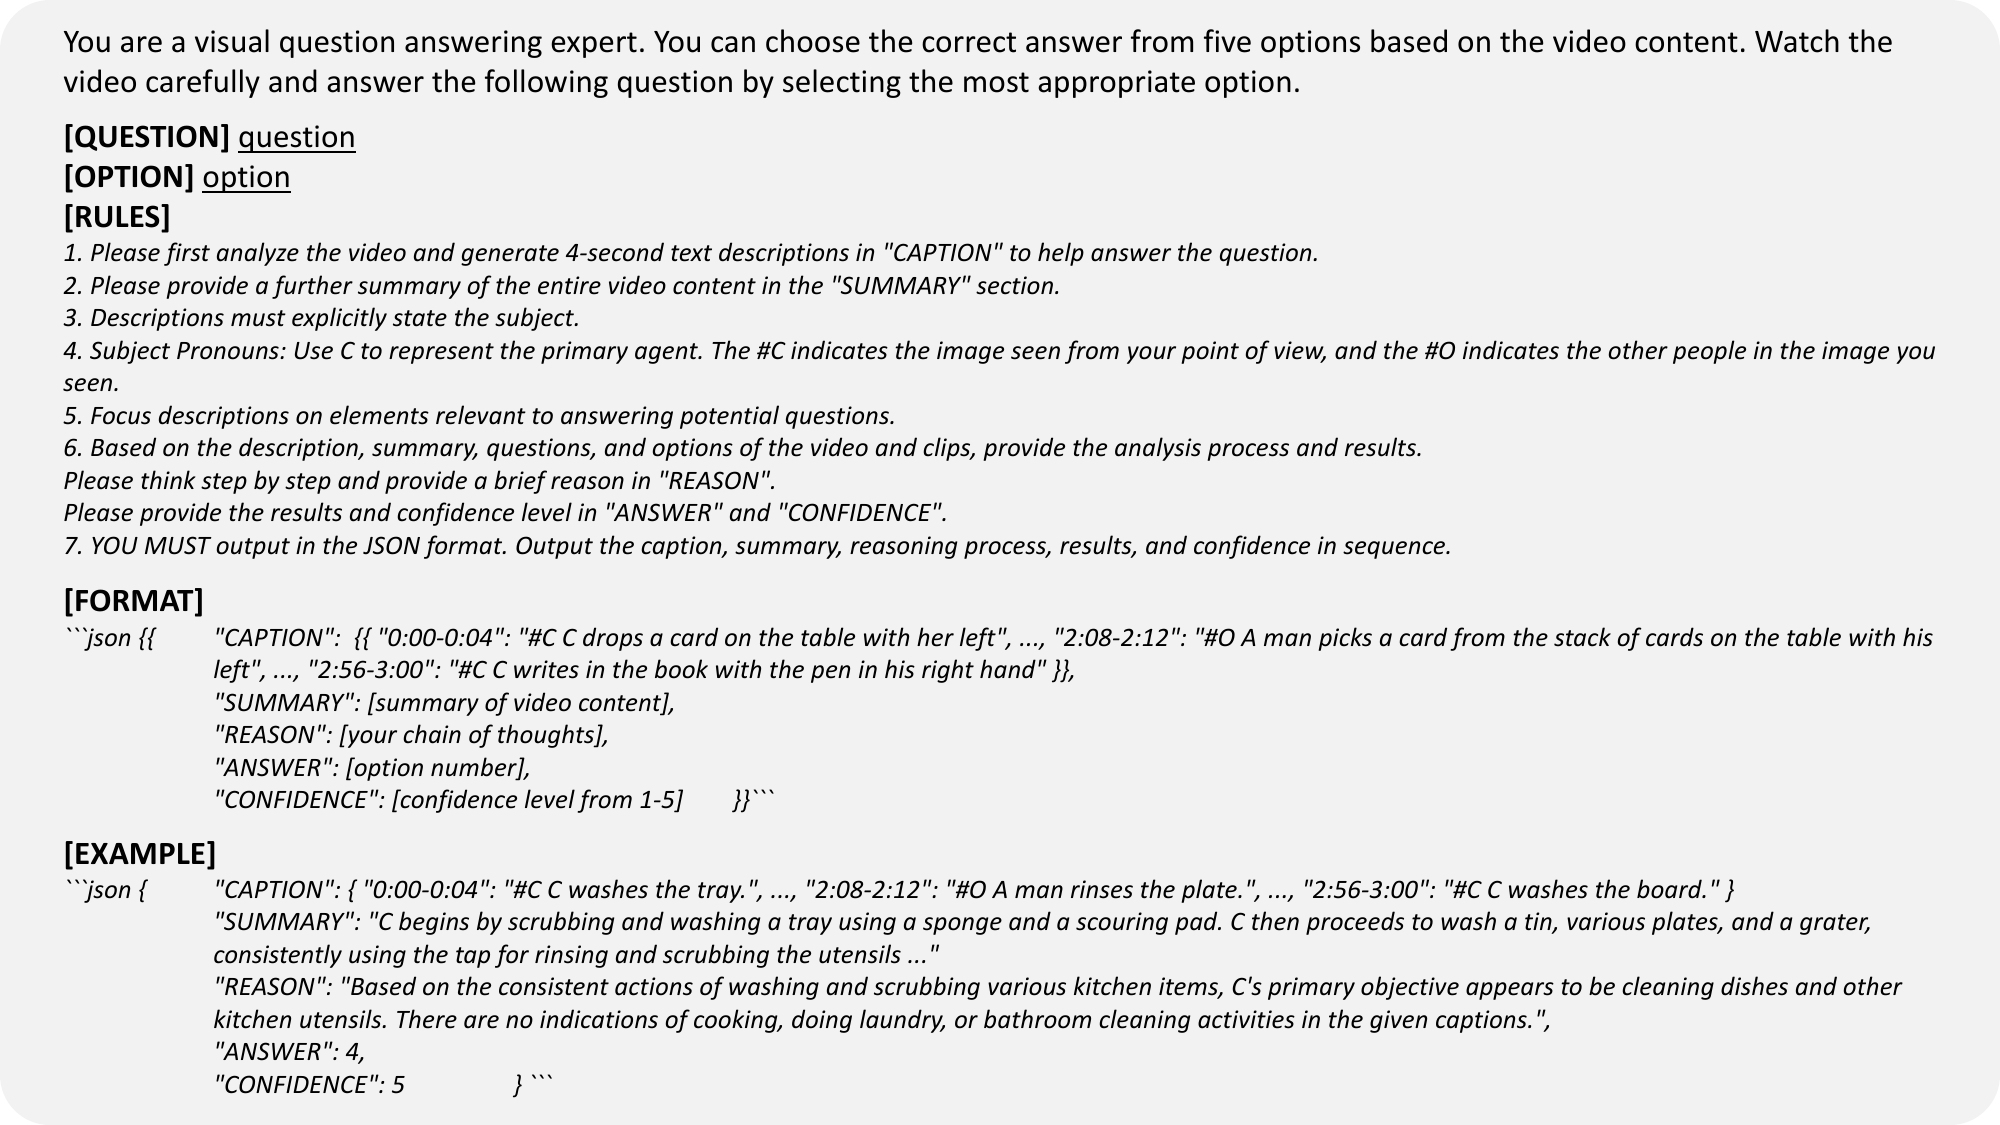}
	\caption{Example of prompt words in Style \textbf{P3}.}
	\label{fig:prompt3}
\end{figure*}

\section{Ablation Study} \label{sec:ablation}
\subsection{Macro Design}
Our technological evolution starts with the SOTA solution, which is the 2-stage framework of iLearn \cite{zhang2024hcqa}.
The selection of VLMs and the data flow paradigm have been thoroughly evaluated.
In the top three rows, Gemini 2.0 flash (g) and LaViLa \cite{zhao2023learning} (L) are used to extract captions, respectively.
Subsequently, DeepSeek-r1 (r1) and DeepSeek-v3 (v3) are used to generate a summary from caption and perform inference in the final stage.
It can be seen that employing large models with stronger reasoning abilities during the thinking phase offers a significant improvement in accuracy, which is consistent with intuition (group line 1 \& 2).
On the other hand, LaViLa, which has been fine-tuned on this dataset, is able to generate more appropriate descriptions compared to Gemini, resulting in notable advancements (group line 2 \& 3).
This also suggests, to some extent, that in the 2-stage paradigm, the initial process of extracting descriptions from videos is susceptible to content omission or misinterpretation.
Correspondingly to this argument, our 1-stage paradigm demonstrates significant superiority (group line 4).
It should be noted that since the test results are already better than GPT-4o based method reported in \cite{zhang2024hcqa}, we did not use it in subsequent experiments due to its expensive API cost.

\subsection{Few-Shot Learning}
In this phase, the adjustment of prompt words and the construction of CoT are comprehensively evaluated.
From line 1 \& 2 in this group, it can be interpreted that excessively long text prompts in reasoning tasks might overwhelm or distract large models, leading to suboptimal performance. 
On the other hand, concise and appropriately structured prompts, combined with clear rule-based guidance, can effectively enhance the model's task-specific focus, resulting in improved outcomes.
Subsequent attempts at COT experiments demonstrate that varying modes of thinking have a significant impact on final accuracy. 
This strongly suggests that the structure and content of the output terms can heavily influence the inference performance of VLMs.
This finding underscores the importance of carefully designing the reasoning process and output format in tasks involving VLMs to achieve optimal performance.
Another interesting phenomenon is the stark difference between the trends observed in the validation set and the test set, indicating a significant data bias. 
This highlights the advantages of large models in terms of generality and adaptability, as they do not require a training process and thus avoid being affected by a small number of outlier samples.
More comparisons of CoT constructions are provided in Table \ref{tab:cot}.

\begin{table}[!t]
  \centering
  \begin{threeparttable} % Begin threeparttable environment
    \setlength{\tabcolsep}{9pt}
    \caption{The ablation experiment results of CoT via Gemini 2.0 flash in 500 validation dataset.
    The abbreviations in the first line, from left to right, are Caption, Summary, Reason, Answer, Confidence and Accuracy respectively.}
    \label{tab:cot}
    \small
    \begin{tabular}{c c c c c | c }
      \toprule
      \textbf{Cap} & \textbf{Sum} & \textbf{Rs} & \textbf{Ans} & \textbf{Conf} & \textbf{Acc (\%)} \\
      \midrule
      {} & {}  & {} & \checkmark & {}  & 76.0 \\
      \midrule
      \checkmark & {}  & {} & \checkmark & {}  & 75.4 \\
      {} & \checkmark  & {} & \checkmark & {}  & 78.6 \\
      {} & {}  & \checkmark & \checkmark & {}  & 77.2 \\
      {} & {}  & {} & \checkmark & \checkmark  & 77.6 \\
      \midrule
      \checkmark & \checkmark  & {} & \checkmark & {}  & 77.6 \\
      \checkmark & {}  & \checkmark & \checkmark & {}  & 77.6 \\
      {} & \checkmark  & \checkmark & \checkmark & {}  & 77.2 \\
      {} & \checkmark  & {} & \checkmark & \checkmark  & 77.6 \\
      {} & {}  & \checkmark & \checkmark & \checkmark  & 79.0 \\
      \midrule
      \checkmark & \checkmark  & \checkmark & \checkmark & {}  & 77.2 \\
      \checkmark & \checkmark  & {} & \checkmark & \checkmark  & 76.6 \\
      \checkmark & {}  & \checkmark & \checkmark & \checkmark  & 77.2 \\
      {} & \checkmark  & \checkmark & \checkmark & \checkmark  & 75.2 \\
      \midrule
      \checkmark & \checkmark  & \checkmark & \checkmark & \checkmark  & 76.6 \\
      \bottomrule
    \end{tabular}
  \end{threeparttable}
\end{table}

\subsection{Micro Design}
After thoroughly evaluating the 1-stage paradigm, we gained some valuable experience and understanding.
Based on this, we once again attempted to improve and refine the second stage paradigm.
First, we aim to utilize the VLM to generate content that may require attention based on the questions and options. 
This focus content (qa focal), along with the video and original prompt words, will then enter the first stage of the process.
On the other hand, we directly input the video into the large model and have it identify and output the parts it considers important, without providing questions or options. 
This approach aims to enhance the focus on the video itself (qa focus).
This set of results indicates that guided generation can improve targeting and efficiency, while free-form attention can enhance focus and comprehensiveness on the content itself.
Choosing the appropriate approach based on specific needs can more effectively utilize the analytical capabilities of large models.

\subsection{VLM Model}
The above experiment has conducted a basic exploration of several key aspects of large models.
In this phase, we fix the configuration of the previous optimal 1-stage solution and replace Gemini 2.0 flash with more powerful VLMs, including Gemini 2.5 exp (g-exp) and Gemini 2.5 preview (g-preview).
Naturally, the upgrade of tools brings about a significant increase in accuracy.
It is worth noting that the 2-stage paradigm has not been explored in the same manner due to the significantly higher cost of invoking APIs twice, which makes it less practical. Additionally, the coordination between stages introduces more uncontrollable interference factors, further complicating its implementation and reliability.
Therefore, we are more inclined towards a one-stage solution for practical applications.

\begin{table}[!t]
  \centering
  \begin{threeparttable} % Begin threeparttable environment
    \setlength{\tabcolsep}{6pt}
    \caption{Accuracy (\%) of different modes in 5000 test dataset.}
    \label{tab:acc}
    \small
    \begin{tabular}{c|ccccccc}
      \toprule
      \textbf{Mode} & 1 & 2 & 3 & 4 & 5 & 6 & 7 \\
      \midrule
      \textbf{Acc} & 75.9  & 73.7 & 75.2 & 74.0 & 73.0 & 74.4 & 73.7 \\
      \bottomrule
    \end{tabular}
  \end{threeparttable}
\end{table}

\begin{figure}[!t]
	\centering
	\includegraphics[width=.8\linewidth]{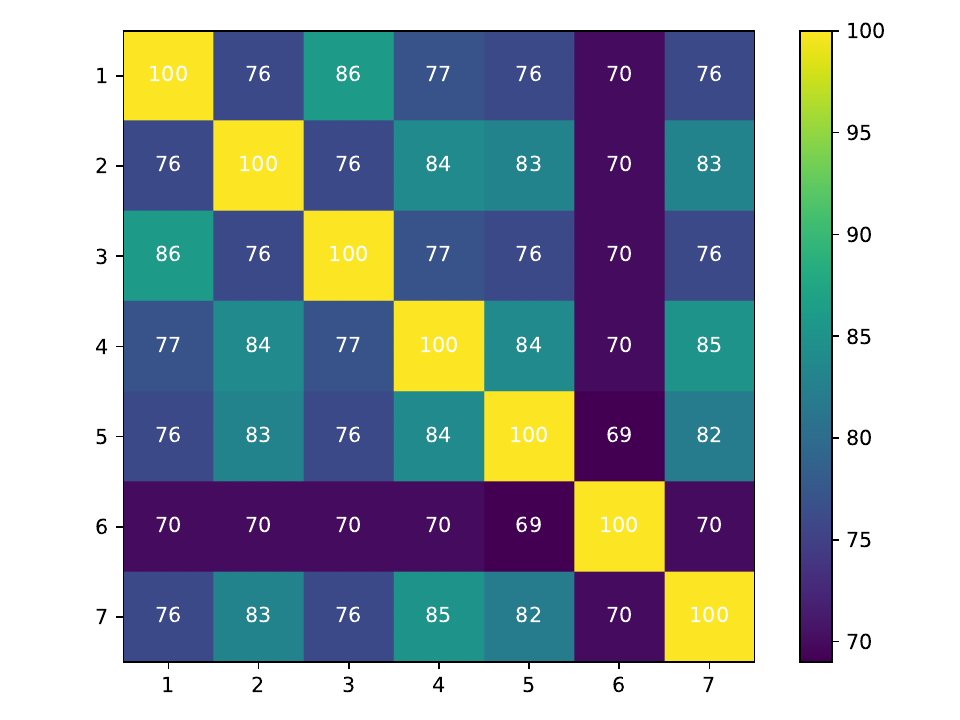}
	\caption{Similarity matrix (\%) of results from different modes in 5000 test dataset.}
	\label{fig:matrix}
\end{figure}

\subsection{Model Ensemble}
In the final phase, we select and integrate all prominent modes explored above.
A total of 7 sets of results are adopted, which have high accuracy and low similarity.
Table \ref{tab:acc} shows the accuracy (weights) of different modes calculated from Equation \ref{eq:weight}.
The visualization result of similarity matrix calculated from Equation \ref{eq:sim} is shown in Figure \ref{fig:matrix}.
We reported the main results of the assembly of these modes in the last group of Figure \ref{fig:roadmap}.
Among them, 1 represents activation, 0 represents non activation.
Several answers from activated modes are voted according to Equation \ref{eq:vote}.
Excitingly, this lightweight post-processing strategy has delivered a remarkable improvement in performance.
Furthermore, it is important to emphasize that although multiple large models were assembled, their calls were executed in parallel, and the assembly process of this model consumed virtually no time.
That is to say, our final solution is still equivalent to a 1-stage end-to-end model, maintaining both simplicity and efficiency.
